# Supplementary material for: Messenger RNA Design via Expected Partition Function and Continuous Optimization
Source: arXiv:2401.00037 source file (2024-03-01)
Supplement: Supplementary file 1 [file appendix.tex]

% !TEX root = main.tex

\section{Comparison of Our Optimization on ncRNA Design with \citet{matthies+:2023}}
\label{sec:appendix_ours_vs_maxs}

Besides the major differences discussed in Section~\ref{sec:related} 
(e.g., our work targets both mRNA  and ncRNA design),
here we compare the technical details of the concurrent work by \citet{matthies+:2023} and our work on ncRNA design (Section~\ref{sec:ncRNA}). For the sake of readability, we use our notations to discuss both their and our work.

Their work optimize a variant of (expected) conditional probability
%our objective 
%$\E_{\vecx\sim \distri(\cdot)} p(\vecy \mid \vecx)$, 
which they define as:
\begin{align}
p(\vecy \mid \distri) 
& \defeq \frac{\expQy (\distri)}{\expQ(\distri)} \\
&= \frac{\E_{\vecx \sim \distri(\cdot)}[e^{-\Delta G(\vecx, \vecy) / RT}]}{\E_{\vecx \sim \distri(\cdot)}[Q(\vecx)]},
\end{align}
where $\expQ_{\vecy} (\distri)$ is interpreted as the expected sequence partition function, representing the weighted sum of Boltzmann weights for all sequences given the fixed structure $\vecy$:
\begin{align}
\expQy (\distri) =  \E_{\vecx \sim \distri(\cdot)}[e^{-\Delta G(\vecx, \vecy) / RT}] = \sum_{\vecx} \distri(\vecx) e^{-\Delta G(\vecx,\vecy) / RT}.
\end{align}

However, it is critical to understand that the objective they proposed differs from the original goal of ncRNA design, which was to optimize:

\begin{align}
 \E_{\vecx \sim \distri(\cdot)}[ p(\vecy \mid \vecx)] = \E_{\vecx \sim \distri(\cdot)} \left [\frac{e^{-\Delta G(x, y) / RT}}{Q(x)} \right ]
 \textcolor{red}{\neq \frac{\E_{\vecx \sim \distri(\cdot)}[e^{-\Delta G(\vecx, \vecy) / RT}]}{\E_{\vecx \sim \distri(\cdot)}[Q(\vecx)]} \defeq p(y \mid \distri)}.
\end{align}

The discrepancy is due to the fact that the expectation of a fraction
is not the fraction of expectations. 
%'s treatment in the formulation, which impacts the optimization objective significantly.

In our work, we directly optimize the expected logarithm of conditional probability:

\begin{align}
 \E_{\vecx \sim \distri(\cdot)}[\log p(\vecy \mid \vecx)] &= \E_{\vecx \sim \distri(\cdot)} \left [\log \left ( \frac{e^{-\Delta G(\vecx, \vecy) / RT}}{Q(\vecx)} \right ) \right ].
\end{align}

Given the complexities in directly optimizing this objective, our proposal includes optimizing a lower bound:

\begin{align}
\E_{\vecx \sim \distri(\cdot)}[\log p(\vecy \mid \vecx)] 
&= \E_{\vecx \sim \distri(\cdot)} \left [\log \left ( \frac{e^{-\Delta G(\vecx, \vecy) / RT}}{Q(\vecx)} \right ) \right ] \\
&= \E_{\vecx \sim \distri(\cdot)} [ -\Delta G(\vecx, \vecy)  / RT - \log Q(\vecx)] \\
&= -\E_{\vecx \sim \distri(\cdot)} [ \Delta G(\vecx, \vecy)  / RT] -  \E_{\vecx \sim \distri(\cdot)}[ \log Q(\vecx)] \\
&\geq -\E_{\vecx \sim \distri(\cdot)} [ \Delta G(\vecx, \vecy)  / RT] -  \textcolor{red}{\log \E_{\vecx \sim \distri(\cdot)}[ Q(\vecx)]}, 
\end{align}
where the inequality applies Jensen's Inequality to the log-expectation term.

In contrast, \citet{matthies+:2023} directly optimized the logarithm of the expected probability without further simplification:

\begin{align}
\log p(\vecy \mid \distri) 
&= \log \left ( \frac{\E_{\vecx \sim \distri(\cdot)}[e^{-\Delta G(\vecx, \vecy) / RT}]}{\E_{\vecx \sim \distri(\cdot)}[Q(\vecx)]} \right )\\
&= \log \E_{\vecx \sim \distri(\cdot)}[e^{-\Delta G(\vecx, \vecy) / RT}] - \log \E_{\vecx \sim \distri(\cdot)}[Q(\vecx)]. 
\end{align}

However, if we apply Jensen's Inequality to the first term of their equation, we will arrive at the same lower bound as our proposal:

\begin{align}
\log p(\vecy \mid \distri)
&\geq  \textcolor{red}{\E_{\vecx \sim \distri(\cdot)}[\log e^{-\Delta G(\vecx, \vecy) / RT}]} - \log \E_{\vecx \sim \distri(\cdot)}[Q(\vecx)] \\
&= - \E_{\vecx \sim \distri(\cdot)}[\Delta G(\vecx, \vecy) / RT] - \log \E_{\vecx \sim \distri(\cdot)}[Q(\vecx)].
\end{align}
